# Supplementary material for: Why Authors Don't Visualize Uncertainty
Source: arXiv:1908.01697 source file (2019-08-05)
Supplement: Supplementary file 1 [file supplement.tex]

https://cran.r-project.org/web/packages/bayesplot/vignettes/graphical-ppcs.html

https://rss.onlinelibrary.wiley.com/doi/pdf/10.1111/rssa.12378

We assume that if a visualization presents a signal, the viewer's visual examination will identify some parameter vector $\theta$ (or set of parameter vectors \jessica{notation}). The parameter of interest could be a slope, a y-intercept, a difference between means, etc.
The viewer will have perceived a discrepancy between the

$T(y)$ -- a vector test statistic
compared to $T(y^rep)$

problem: assumes identical perceivers (similar limitation to original LineUps proposal)

heterogeneity of

now T(y) (or perceived T(y)) is drawn from

The focus of Buja, Cook, Wickham and others is class of null hypotheses that can be easily simulated via permutation of the observed data, even in the absence of randomization or a probability model. For Gelman the replication distribution is represented by several plots representing simulations of the original graphic, depicting replicated datasets if the model were true. If the visual inspection of the data (T(y)) shows patterns that don't appear in the replications, then the exploratory analysis has indicated a potential

Buja 1999 
- scenario where the feature is absent = null distribution
- underlying feature = a specific alternative
- visible feature = a statistical test

Visual feature detector = test function (data) such that
-(data) = 1 if a feature is detected,
-(data) = 0 if no feature is detected.

Buja et al. 1999 suggest that the presence (or absence) of features usually needs no testing, 
presence/absence of features usually needs no testing; tests are needed when in doubt that a feature is present or absent.
(this statement assumes a given visual feature detector)

When a 1 is returned -- doesn't allow for confidence

Gelman 2004 - 
Leaves the process by which a discrepancy is idnetified between the test statistic (vis) and $T(y^rep)$

The test statistic has some magnitude that can be evaluated for strength.

Buja 2009
